# Supplementary material for: Level Set Learning for Poincar\'e Plots of Symplectic Maps
Source: arXiv:2312.00967 source file (2023-12-01)
Supplement: Supplementary file 1 [file 10_Appendix.tex]

\section{Higher Order Eigenfunctions}
\label{app:higher-order-eigenfunctions}
\begin{figure}
    \centering
    \includegraphics[width=0.8\textwidth]{tex/KernelLabel/Figures/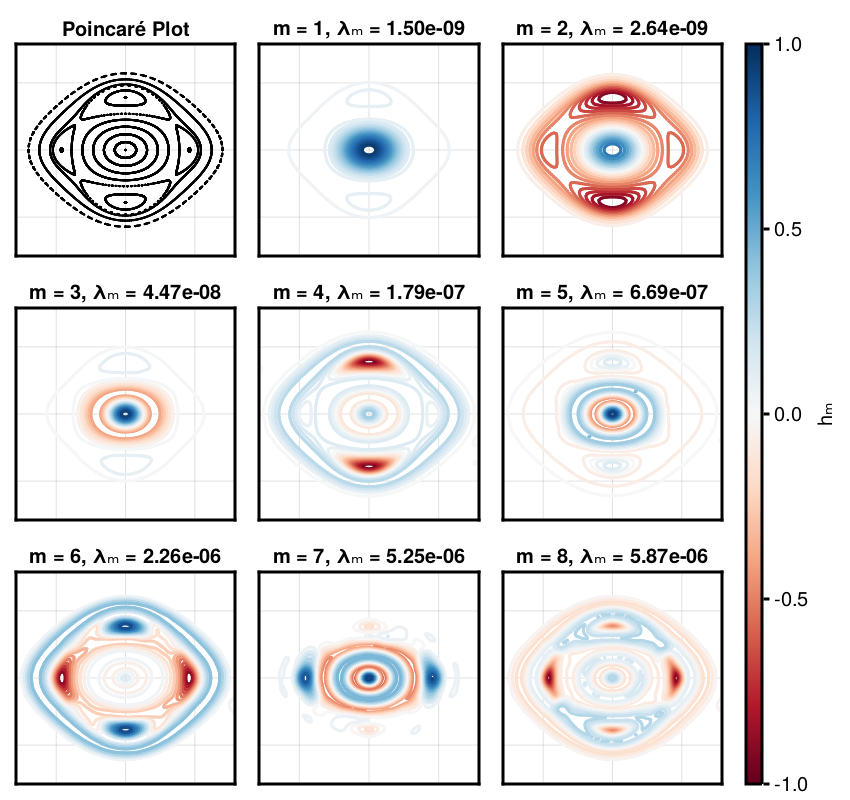}
    \caption{A Poincar\'e plot and the lowest eight eigenmodes and eigenvalues of the perturbed pendulum example \cref{eq:perturbed-pendulum}. }
    \label{fig:eigenvectors}
\end{figure}

In this appendix, we show an example of higher order eigenfunctions of the Rayleigh quotient method. 
For the example, we consider the 1.5D Hamiltonian system of a perturbed pendulum used in \cite{Burby2021, Rath2021}
\begin{gather}
\label{eq:perturbed-pendulum}
    H_{\rm pp}(x, y, t) = \frac{1}{2} y^2 - \frac{1}{4} \cos x - \frac{1}{20}\left[3 x y \sin (2t) + 0.7 x y \sin(3t) \right], \\
    \dot x = \pd{H_{\rm pp} }{y}, \qquad \dot y = - \pd{H_{\rm pp}}{x}. 
\end{gather}
A symplectic map is obtained by evolving a trajectory from $t=0$ to $t=2\pi$, i.e.~$\sympmap : (x(0), y(0)) \mapsto (x(2\pi), y(2\pi))$.
We use the inverse multiquadric kernel \eqref{eq:inversemultiquadric} with $\sigma = 0.25$. 
For the domain, we choose $\Omega = [-0.79, 0.79] \times [-0.79, 0.79]$ and boundary conditions $\Gamma = \Rbb^2 \backslash \left( [-0.75, 0.75] \times [-0.75, 0.75] \right)$ and let $\wbd = \mathbbm{1}_\Gamma$. 
We use $N = 1000$ points, $\epsilon = 10^{-8}$, and solve for $8$ eigenvalues and eigenvectors.
 
In \cref{fig:eigenvectors}, we show Poincar\'e plot and the lowest eight eigenfunctions.
The eigenvalues (shown in titles) vary from $1.5 \times 10^{-9}$ to $5.87 \times 10^{-6}$, indicating how the functions violate our energies more and more.
The lowest order mode concentrates its mass on the largest region of nested circles.
As the mode number $m$ increases, we see the modes become increasingly oscillatory. 
Additionally, some higher order modes ($m=4, 6, 7$) emphasize the islands more than the core.
The first few eigenmodes ($m\leq 5$) are visually invariant, while the $m\geq 6$ modes have more visible signs of invariance.
